# Supplementary material for: Interactive Visualization for Debugging RL
Source: arXiv:2008.07331 source file (2020-08-18)
Supplement: Supplementary file 1 [file appendix.tex]

\section*{Appendix}

\textsc{Visualizations}

\begin{figure}[h]
    \centering
    \includegraphics[width=\linewidth]{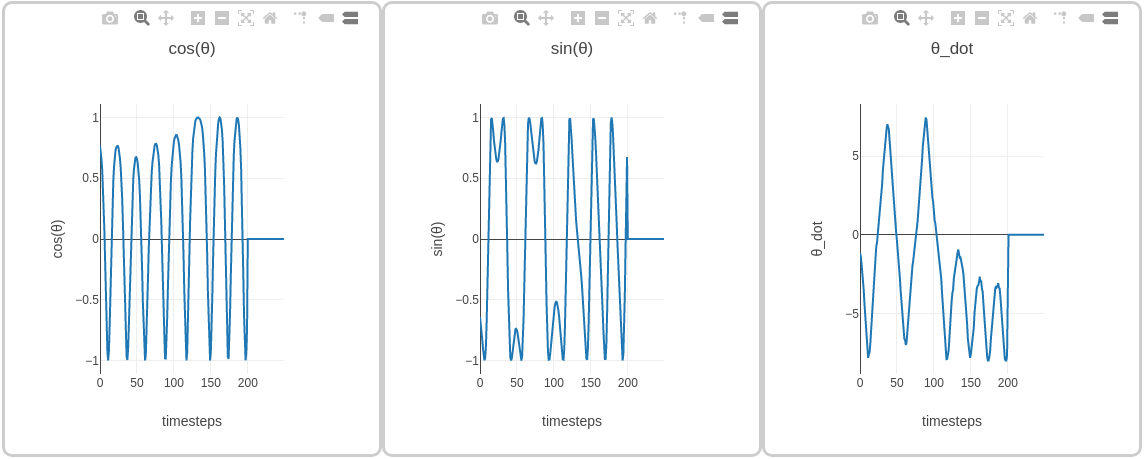}
    \vspace{-0.5em}
    \caption{\textbf{State Viewport}:
    \small
    Visualizing state viewports for the inverted pendulum task. This representation with a generated state viewport backed by an image buffer spec (see Figure \ref{fig:action_space}), provides the user with better intuition about the correspondence between states and actions for non image state spaces, which is easier to interpret.}
    \label{fig:state_space_viewport}
    \vspace{-1em}
\end{figure}

\begin{figure}[h]
    \centering
    \includegraphics[width=\linewidth]{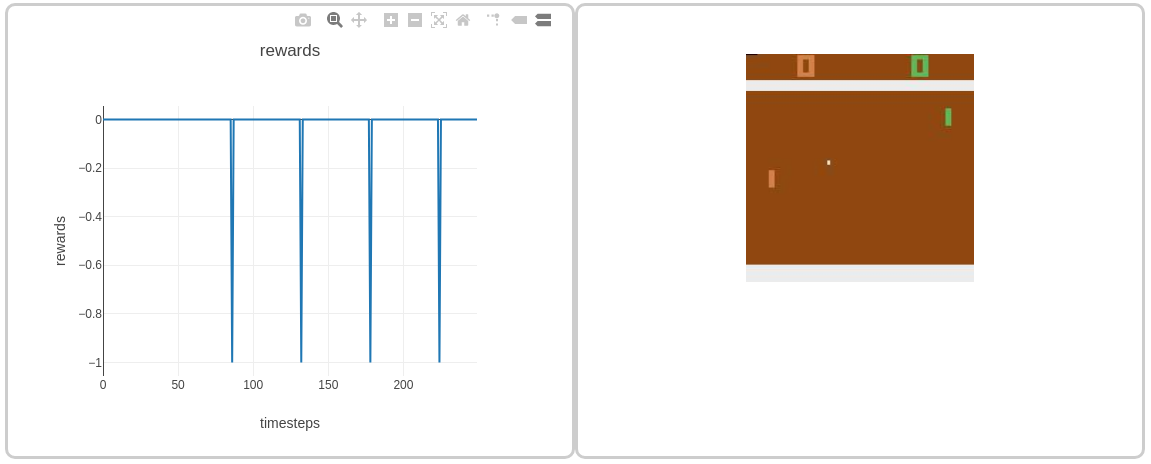}
    \caption{\textbf{Reward + State Space Viewport} 
    \small
    Visualizing reward \& state space viewports for the Pong environment \cite{bellemare_arcade_2013}. This representation provides the user with a better intuition about the correspondence between rewards and states, especially for environments with denser rewards.
    }
    \label{fig:reward_plot}
    \vspace{-1em}
\end{figure}
